# Supplementary material for: Quantum many-body scars in bipartite Rydberg arrays originate from hidden projector embedding
Source: arXiv:2203.00658 source file (2022-12-12)
Supplement: Supplementary file 1 [file appendix.tex]

\section{Another proof of known exact eigenstates}
There are several exact eigenstates known in PXP model, which was found in Ref.~\cite{Lin2019mps}. They are one zero-energy eigenstate for periodic boundary condition (PBC), and four eigenstates for open boundary condition (OBC). Their wave functions were originally given as matrix product states (MPS), and it was pointed out that a certain basis transformation connect the zero energy eigenstate to the ground state of AKLT model. Later, Ref.~\cite{Shiraishi_2019} gave an elegant proof of the zero energy state, by showing that the basis transformation yields a form $H=\sum_i\mc{P}_ih_i\mc{P}_i+H'$ where $\mc{P}_i$ is a local projection operator. This form is known as Shiraishi-Mori form, which provided a systematic recipe to construct models that violate ETH~\cite{mori_shiraishi}.   

In this section, we provided another proof of these exact eigenstates based on the basis transformation in the main text.
\subsection{Fractionalization}
In order to do so, we introduce a notion of fractionalizing the $N$ spin-$1$ particles into $2N$ spin-$1/2$ particles. We define a map $A_b:\mb{C}^{2\otimes2}\rightarrow\mb{C}^3$ for $\forall b\in\Lambda_{\mr{B}}$:
\begin{equation}
    A_b\coloneqq\ket*{+}_b\bra*{\uparrow\uparrow}_{(b,\mr{L}),(b,\mr{R})}+\ket*{0}_b\frac{1}{\sqrt{2}}\left(\bra*{\uparrow\downarrow}+\bra*{\downarrow\uparrow}\right)_{(b,\mr{L}),(b,\mr{R})}+\ket*{-}_b\bra*{\downarrow\downarrow}_{(b,\mr{L}),(b,\mr{R})},
\end{equation}
where $(b,\mr{L/R})\in\Lambda_{\mr{B}}^{\mr{frac}}\coloneqq\Lambda_{\mr{B}}\times\{\mr{L},\mr{R}\}$ is a lattice site for ``fractional" spin-$1/2$s. Physical meaning of this map is to regard one particle with spin-$1$ as a composite state of two particles with spin-$1/2$, which can be done by discarding the singlet component. We also define a product of such a map as $\msf{A}\coloneqq\prod_{b\in\Lambda_{\mr{B}}}A_b:\mb{C}^{2\otimes2\otimes N}\rightarrow\mb{C}^{3\otimes N}$.  

We can also fractionalize the spin operator with $S=1$ in a sense that for an arbitrary operator $O$ of $S=1$, there exists an operator $O_{\mr{frac}}:\mb{C}^{2\otimes2}\rightarrow\mb{C}^{2\otimes}$ such that $O\msf{A}=\msf{A}O_{\mr{frac}}$. The choice of $O_{\mr{frac}}$ is not unique. For example, both operators $\sqrt{2}\dyad*{\uparrow\uparrow}{\uparrow\downarrow}_{(b,\mr{L}),(b,\mr{R})}$ and $\sqrt{2}\dyad*{\uparrow\uparrow}{\downarrow\uparrow}_{(b,\mr{L}),(b,\mr{R})}$ correspond to $\dyad*{+}{0}$. However, there is a natural choice for $O_{\mr{frac}}$: we first note that for any operator-valued function $F$, it holds that
\begin{equation}\label{eq:operator identity}
    F(\{\bm{S}_b\}_{b\in\Lambda_{\mr{B}}})\msf{A}=\msf{A}F\left(\left\{\bm{S}_{(b,\mr{L})}+\bm{S}_{(b,\mr{R})}\right\}_{b\in\Lambda_{\mr{B}}}\right),
\end{equation}
where $\bm{S}_b$ is a spin operator with $S=1$, i.e., $\bm{S}_b:\mb{C}^3\rightarrow\mb{C}^3$, and $\bm{S}_{(b,\mr{L/R})}$ is a spin operator with $S=1/2$, i.e., $\bm{S}_{(b,\mr{L/R})}:\mb{C}^2\rightarrow\mb{C}^2$. This is physically quite natural, as the spin operator $\bm{S}_b$ is split into a sum of two spin operators $\bm{S}_{(b,\mr{L})}+\bm{S}_{(b,\mr{R})}$.
\subsection{Defining exact eigenstates}
We consider the following states for one zero energy eigenstate $\ket*{\Gamma}$ with PBC and for four eigenstates $\ket*{\Gamma^{\tau\tau'}}$ with OBC:
\begin{equation}\label{eq:|Gamma> in SM}
    \begin{split}
        \ket*{\Gamma}&=\msf{A}\bigotimes_{b\in\Lambda_{\mr{B}}}\frac{1}{\sqrt{2}}\left(\ket*{\uparrow\uparrow}-\ket*{\downarrow\downarrow}\right)_{(b,\mr{R}),(b+1,\mr{L})}\\
        \ket*{\Gamma^{\tau\tau'}}&=\msf{A}\bigotimes_{b\in\Lambda_{\mr{B}}\setminus\{N\}}\frac{1}{\sqrt{2}}\left(\ket*{\uparrow\uparrow}-\ket*{\downarrow\downarrow}\right)_{(b,\mr{R}),(b+1,\mr{L})}\otimes\ket*{\tau}_{(1,\mr{L})}\ket*{\tau'}_{(N,\mr{R})},
    \end{split}
\end{equation}
where $\ket*{\tau}$ and $\ket*{\tau'}$ are either $\ket*{\rightarrow}\coloneqq(\ket*{\uparrow}+\ket*{\downarrow})/\sqrt{2}$ or $\ket*{\leftarrow}\coloneqq(\ket*{\uparrow}-\ket*{\downarrow})/\sqrt{2}$, namely eigenstates of $X$. A pictorial representation of them is described in Fig.~[FIG]. 

We first show that they are elements of $\mc{V}_{\mr{Ryd}}$. To do so, we consider the following state:
\begin{equation}
    \ket*{\gamma^{\sigma\sigma'}_{b,b+1}}\coloneqq \ket{\sigma}_{(b,\mr{L})}\frac{1}{\sqrt{2}}\left(\ket{\uparrow\uparrow}-\ket{\downarrow\downarrow}\right)_{(b,\mr{R}),(b+1,\mr{L})}\ket*{\sigma'}_{b+1,\mr{R}},
\end{equation}
where $\sigma$ and $\sigma'$ are either $\uparrow$ or $\downarrow$, namely eigenstates of  $Z$. Note that $\ket*{\Gamma}$ and $\ket*{\Gamma^{\tau\tau'}}$ are superpositions of $\ket*{\gamma^{\sigma\sigma'}_{b,b+1}}$ in a sense that for $\forall b\in\Lambda_{\mr{B}}$, one can express them as 
\begin{equation}\label{eq:|Gamma> decomposition}
    \begin{split}
         \ket*{\Gamma}&=\msf{A}\sum_{\sigma,\sigma'=\uparrow,\downarrow}c_{\sigma\sigma'}\ket*{\gamma^{\sigma\sigma'}_{b,b+1}}\otimes\ket*{\Xi_{\sigma\sigma'}}\\
         \ket*{\Gamma^{\tau\tau'}}&=\msf{A}\sum_{\sigma,\sigma'=\uparrow,\downarrow}c_{\sigma\sigma'}\ket*{\gamma^{\sigma\sigma'}_{b,b+1}}\otimes\ket*{\Xi^{\tau\tau'}_{\sigma\sigma'}},
    \end{split}
\end{equation}
where $c_{\sigma\sigma'}$ is a coefficient and $\ket*{\Xi_{\sigma\sigma'}}$ and $\ket*{\Xi_{\sigma\sigma'}^{\tau\tau'}}$ are spin-$1/2$ states defined on $(\Lambda_{\mr{B}}\setminus\{b,b+1\})\times\{\mr{L},\mr{R}\}$.
A straightforward calculation yields
\begin{equation}
    \begin{split}
        A_b\otimes A_{b+1}\ket*{\gamma_{b,b+1}^{\uparrow\uparrow}}&=\frac{1}{\sqrt{2}}\ket*{+,+}_{b,b+1}-\frac{1}{2\sqrt{2}}\ket*{0,0}_{b,b+1}\\
        A_b\otimes A_{b+1}\ket*{\gamma_{b,b+1}^{\uparrow\downarrow}}&=\frac{1}{2}\ket*{+,0}_{b,b+1}-\frac{1}{2}\ket*{0,-}_{b,b+1}\\
        A_b\otimes A_{b+1}\ket*{\gamma_{b,b+1}^{\downarrow\uparrow}}&=\frac{1}{2}\ket*{0,+}_{b,b+1}-\frac{1}{2}\ket*{-,0}_{b,b+1}\\
        A_b\otimes A_{b+1}\ket*{\gamma_{b,b+1}^{\downarrow\downarrow}}&=\frac{1}{2\sqrt{2}}\ket*{0,0}_{b,b+1}-\frac{1}{\sqrt{2}}\ket*{-,-}_{b,b+1}.
    \end{split}
\end{equation}
Therefore, combined with Eq.~\eqref{eq:|Gamma> decomposition}, one finds 
\begin{equation}\label{eq:local Pryd}
    \begin{split}
        (1-\dyad{+,-})_{b,b+1}\ket*{\Gamma}&=+\ket*{\Gamma}\\
        (1-\dyad{+,-})_{b,b+1}\ket*{\Gamma^{\tau\tau'}}&=+\ket*{\Gamma^{\tau\tau'}}
    \end{split}
\end{equation}
for $\forall b\in\Lambda_{\mr{B}}$. Since $P_{\mr{Ryd}}$ is a product of $\left(1-\dyad{+,-}\right)_{b,b+1}$ and $\left[(1-\dyad{+,-})_{b,b+1},(1-\dyad{+,-})_{b',b'+1}\right]=0$ for $\forall b,b'\in\Lambda_{\mr{B}}$, namely local constraints commute with each other, we find $P_{\mr{Ryd}}\ket*{\Gamma}=+\ket*{\Gamma}$ and $P_{\mr{Ryd}}\ket*{\Gamma^{\tau\tau'}}=+\ket*{\Gamma^{\tau\tau'}}$. This means $\ket*{\Gamma},\ket*{\Gamma^{\tau\tau'}}\in\mc{V}_{\mr{Ryd}}$.
\subsection{A detailed proof of exact eigenstates}
As $P_{\mr{Ryd}}\ket*{\Gamma}=+\ket*{\Gamma}$, it holds that
\begin{equation}
    H\ket*{\Gamma}=HP_{\mr{Ryd}}\ket*{\Gamma}=P_{\mr{Ryd}}H\ket*{\Gamma}=P_{\mr{Ryd}}\left(H_{\mr{Z}}+H_1\right)\ket*{\Gamma}.
\end{equation}
Here we use $\left[P_{\mr{Ryd}},H\right]=0$ and $P_{\mr{Ryd}}\dyad*{+,-}{\psi}_{b,b+1}=0$ for $\forall\ket{\psi}\in\mb{C}^{3\otimes2}$. Also, Eq.~\eqref{eq:local Pryd} implies that $\dyad*{\psi}{+,-}_{b,b+1}\ket*{\Gamma}=0$ for $\forall b\in\Lambda_{\mr{B}}$. Thus, we obtain $H\ket*{\Gamma}=P_{\mr{Ryd}}H_{\mr{Z}}\ket*{\Gamma}$.
The same relation holds for $\ket*{\Gamma^{\tau\tau'}}$ as well. With the operator identity in Eq.~\eqref{eq:operator identity}, we find
\begin{equation}\begin{split}
    H_{\mr{Z}}\ket{\Gamma}&=\msf{A}\left(\sqrt{2}\sum_{b\in\Lambda_{\mr{B}}}\left(\frac{1}{2}X_{(b,\mr{L})}+\frac{1}{2}X_{(b,\mr{R})}\right)\right)\bigotimes_{b'\in\Lambda_{\mr{B}}}\frac{1}{\sqrt{2}}\left(\ket{\uparrow\uparrow}-\ket{\downarrow\downarrow}\right)_{(b',\mr{R}),(b'+1,\mr{L})}\\
    &=\msf{A}\left(\sqrt{2}\sum_{b\in\Lambda_{\mr{B}}}\left(\frac{1}{2}X_{(b,\mr{R})}+\frac{1}{2}X_{(b+1,\mr{L})}\right)\right)\bigotimes_{b'\in\Lambda_{\mr{B}}}\frac{1}{\sqrt{2}}\left(\ket{\uparrow\uparrow}-\ket{\downarrow\downarrow}\right)_{(b',\mr{R}),(b'+1,\mr{L})}\\&=0,
    \end{split}
\end{equation}
where PBC is used in the second line. For $\ket*{\Gamma^{\tau\tau'}}$, we find
\begin{equation}
    \begin{split}
        H_{\mr{Z}}\ket*{\Gamma^{\tau\tau'}}&=\msf{A}\left(\sqrt{2}\sum_{b\in\Lambda_{\mr{B}}}\left(\frac{1}{2}X_{(b,\mr{L})}+\frac{1}{2}X_{(b,\mr{R})}\right)\right)\bigotimes_{b'\in\Lambda_{\mr{B}}\setminus\{N\}}\frac{1}{\sqrt{2}}\left(\ket*{\uparrow\uparrow}-\ket*{\downarrow\downarrow}\right)_{(b',\mr{R}),(b'+1,\mr{L})}\otimes\ket*{\tau}_{(1,\mr{L})}\ket*{\tau'}_{(N,\mr{R})}\\
        &=\msf{A}\frac{1}{\sqrt{2}}\left(X_{(1,\mr{L})}+X_{(N,\mr{R})}\right)\bigotimes_{b'\in\Lambda_{\mr{B}}\setminus\{N\}}\frac{1}{\sqrt{2}}\left(\ket*{\uparrow\uparrow}-\ket*{\downarrow\downarrow}\right)_{(b',\mr{R}),(b'+1,\mr{L})}\otimes\ket*{\tau}_{(1,\mr{L})}\ket*{\tau'}_{(N,\mr{R})}.
    \end{split}
\end{equation}
As $\ket{\tau}$ and $\ket*{\tau'}$ are eigenstates of $X$, $\ket*{\Gamma^{\tau\tau'}}$ is also an eigenstate of $H_{\mr{Z}}$.
\subsection{Matrix product state representation}
In Ref.~\cite{Lin2019mps}, the zero energy eigenstate for PBC and four eigenstates for OBC are given as matrix product states (MPS). We re-derive MPS representation of $\ket*{\Gamma}$ and $\ket*{\Gamma^{\tau\tau'}}$ and show an equivalence between the states considered in Ref.~\cite{Lin2019mps} and the states in Eq.~\eqref{eq:|Gamma> in SM}. To do so, we define a bond variable $\rket{\alpha}_b$ %:\{1,2\}\rightarrow\{\ket*{\uparrow\uparrow}_{(b-1,\mr{R}),(b,\mr{L})},\ket*{\downarrow\downarrow}_{(b-1,\mr{R}),(b,\mr{L})}\}$
for $b\in\Lambda_{\mr{B}}$ such that
\begin{equation}
    \rket{0}_b\coloneqq\ket*{\uparrow\uparrow}_{(b-1,\mr{R}),(b,\mr{L})},\,\,
    \rket{1}_b\coloneqq\ket*{\downarrow\downarrow}_{(b-1,\mr{R}),(b,\mr{L})}.
\end{equation}
$\ket*{\Gamma}$ is re-written as
\begin{equation}
    \begin{split}
        \ket*{\Gamma}&=\msf{A}\bigotimes_{b\in\Lambda_{\mr{B}}}\frac{1}{\sqrt{2}}\left(\rket{0}-\rket{1}\right)_b.
    \end{split}
\end{equation}
From this expression, we can find MPS representation for $\ket*{\Gamma}$: a straightforward calculation yields
\begin{equation}\begin{split}
    A_b\frac{1}{\sqrt{2}}\left(\rket{0}-\rket{1}\right)_b\otimes\frac{1}{\sqrt{2}}\left(\rket{0}-\rket{1}\right)_{b+1}&=\msf{A}_{1,1}^+\ket*{\uparrow}_{(b-1,\mr{R})}\ket*{+}_b\ket*{\uparrow}_{(b+1,\mr{L})}+\msf{A}_{1,2}^0\ket*{\uparrow}_{(b-1,\mr{R})}\ket*{0}_b\ket*{\downarrow}_{(b+1,\mr{L})}\\
    &-\msf{A}_{2,1}^0\ket*{\downarrow}_{(b-1,\mr{R})}\ket*{0}^b\ket*{\uparrow}_{(b+1,\mr{L})}-\msf{A}_{2,2}^-\ket*{\downarrow}_{(b-1,\mr{R})}\ket*{-}_b\ket*{\downarrow}_{(b+1,\mr{L})},
    \end{split}
\end{equation}
where 
\begin{equation}
\msf{A}_{1,1}^+\coloneqq\frac{1}{2},\,\,\msf{A}^0_{1,2}\coloneqq-\frac{1}{2\sqrt{2}},\,\,\msf{A}^0_{2,1}\coloneqq\frac{1}{2\sqrt{2}},\,\,\msf{A}^-_{2,2}\coloneqq-\frac{1}{2}.
\end{equation}
Therefore, $\ket*{\Gamma}$ is written as
\begin{equation}
    \ket*{\Gamma}=\sum_{\{\sigma_i\}_{i=1}^N\in\{\pm,0\}^{\otimes N}}\mr{Tr}\left[\msf{A}^{\sigma_1}\cdots\msf{A}^{\sigma_{N}}\right]\ket*{\sigma_1\cdots\sigma_N},
\end{equation}
where 
\begin{equation}
    \msf{A}^+\coloneqq\frac{1}{2\sqrt{2}}\begin{pmatrix}\sqrt{2} & 0\\0&0\end{pmatrix},\,\,\msf{A}^0\coloneqq\frac{1}{2\sqrt{2}}\begin{pmatrix}0&-1\\1&0\end{pmatrix},\,\,\msf{A}^-\coloneqq\frac{1}{2\sqrt{2}}\begin{pmatrix}0&0\\0&-\sqrt{2}\end{pmatrix}.
\end{equation}
Up to an irrelevant normalization factor, this is the same as the zero energy state in Ref.~\cite{Lin2019mps}.

A similar consideration leads to MPS representation of $\ket*{\Gamma^{\tau\tau'}}$:
\begin{equation}
    \begin{split}
        \ket*{\Gamma^{\tau\tau}}=\sum_{\{\sigma_i\}_{i=1}^N\in\{\pm,0\}^{\otimes N}}\left(\msf{v}_\tau^{\sigma_1}\right)^{\mr{T}}\msf{A}^{\sigma_2}\cdots\msf{A}^{\sigma_{N-1}}\msf{w}_{\tau'}^{\sigma_N}\ket*{\sigma_1\cdots\sigma_N},
    \end{split}
\end{equation}
where 
\begin{equation}
    \begin{split}
        \msf{v}_\rightarrow^+&\coloneqq\frac{1}{2}\begin{pmatrix}\sqrt{2}\\0\end{pmatrix},\,\,\msf{v}_\rightarrow^0\coloneqq\frac{1}{2}\begin{pmatrix}1\\-1\end{pmatrix},\,\,\msf{v}_\rightarrow^-\coloneqq\frac{1}{2}\begin{pmatrix}0\\-\sqrt{2}\end{pmatrix},\,\,\msf{v}^+_\leftarrow\coloneqq\frac{1}{2}\begin{pmatrix}\sqrt{2}\\0\end{pmatrix},\,\,\msf{v}^0_\leftarrow\coloneqq\frac{1}{2}\begin{pmatrix}-1\\-1\end{pmatrix},\,\,\msf{v}_\leftarrow^-\coloneqq\frac{1}{2}\begin{pmatrix}0\\\sqrt{2}\end{pmatrix},\\
        \msf{w}_\rightarrow^+&\coloneqq\frac{1}{2\sqrt{2}}\begin{pmatrix}\sqrt{2}\\0\end{pmatrix},\,\,\msf{w}_\rightarrow^0\coloneqq\frac{1}{2\sqrt{2}}\begin{pmatrix}1\\1\end{pmatrix},\,\,\msf{w}_\rightarrow^-\coloneqq\frac{1}{2\sqrt{2}}\begin{pmatrix}0\\\sqrt{2}\end{pmatrix},\,\,\msf{w}_\leftarrow^+\coloneqq\frac{1}{2\sqrt{2}}\begin{pmatrix}\sqrt{2}\\0\end{pmatrix},\,\,\msf{w}_\leftarrow^0\coloneqq\frac{1}{2\sqrt{2}}\begin{pmatrix}-1\\1\end{pmatrix},\,\,\msf{w}_\leftarrow^-\coloneqq\frac{1}{2\sqrt{2}}\begin{pmatrix}0\\-\sqrt{2}\end{pmatrix}.
    \end{split}
\end{equation}
Since one can find
\begin{equation}\begin{split}
\begin{pmatrix}1&1\end{pmatrix}\msf{A}^\sigma&=\frac{1}{\sqrt{2}}\msf{v}^\sigma_\rightarrow,\,\,\begin{pmatrix}1&-1\end{pmatrix}\msf{A}^\sigma=\frac{1}{\sqrt{2}}\msf{v}^\sigma_\leftarrow,\,\,\msf{A}^\sigma\begin{pmatrix}1\\1\end{pmatrix}=\msf{w}^\sigma_\leftarrow,\,\,\msf{A}^\sigma\begin{pmatrix}1\\-1\end{pmatrix}=\msf{w}^\sigma_\rightarrow,
\end{split}
\end{equation}
this is equivalent to four states in Ref.~\cite{Lin2019mps}.
%Note that we have
%\begin{equation}\begin{split}
    %A_b\rket{1,1}_{b,b+1}&=\ket*{\uparrow}_{(b-1,\mr{R})}\ket*{+}_b\ket*{\uparrow}_{(b+1,\mr{L})},\,\,A_b\rket{1,2}_{b,b+1}=\ket*{\uparrow}_{(b-1,\mr{R})}\frac{1}{\sqrt{2}}\ket*{0}_b\ket*{\downarrow}_{(b+1,\mr{L})}\\
    %A_b\rket{2,1}_{b,b+1}&=\ket*{\downarrow}_{(b-1,\mr{R})}\frac{1}{\sqrt{2}}\ket*{0}_b\ket*{\uparrow}_{(b+1,\mr{L})},\,\,A_b\rket{2,2}_{b,b+1}=\ket*{\downarrow}_{(b-1,\mr{R})}\ket*{-}_b\ket*{\downarrow}_{(b+1,\mr{L})}.
    %\end{split}
%\end{equation}
%an operator $B:\{1,2\}\times\{1,2\}\rightarrow\mb{C}^3$ such that
%\begin{equation}
    %B(1,1)=A_b
%\end{equation}
\section{A detailed derivation of the energy of the scar states}
Here we provide a detailed derivation of the estimate of the energy of the scar states $\ket*{\mc{S}_{N}}$ and $\ket*{\mc{S}_{N-1}}$. Our trial wave functions corresponding to these states are as follows:
\begin{equation}
    \ket*{S_N}=P_{\mr{Ryd}}\bigotimes_{b\in\Lambda_{\mr{B}}}\ket*{\what{+}}_b, \,\,\ket*{S_{N-1}}=\sqrt{2}\sum_{b\in\Lambda_{\mr{B}}}P_{\mr{Ryd}}\ket*{\what{0}}_b\bigotimes_{b'\in\Lambda_{\mr{B}}\setminus\{b\}}\ket*{\what{+}}_{b'}.
\end{equation}
We find
\begin{equation}
    \begin{split}
        H\ket*{S_N}=P_{\mr{Ryd}}\left(H_{\mr{Z}}+H_1\right)\ket*{\wtil{S}_N}=N\sqrt{2}\ket*{S_N}-\frac{1}{4}\sum_{b\in\Lambda_{\mr{B}}}P_{\mr{Ryd}}\left(\ket*{+,0}+\ket*{0,-}\right)_{b,b+1}\bigotimes_{b'\in\Lambda_{\mr{B}}\setminus\{b,b+1\}}\ket*{\what{+}}_{b'}.
    \end{split}
\end{equation}
We express $\ket*{+,0}+\ket*{0,-}$ in the $S^x$ basis $\ket*{\what{\pm}}, \ket*{\what{0}}$,
\begin{equation}
    \begin{split}
        \ket*{+,0}+\ket*{0,-}&=\frac{1}{\sqrt{2}}\ket*{\what{+},\what{+}}-\frac{1}{\sqrt{2}}\ket*{\what{T}_{1,1}}-\frac{1}{\sqrt{2}}\ket*{\what{T}_{1,-1}}-\frac{1}{\sqrt{2}}\ket*{\what{-},\what{-}},
    \end{split}
\end{equation}
where $\ket*{\what{T}_{S,M}}$ is a composite state with total spin $S$ and $S^x=M$. Thus we obtain
\begin{equation}
    -\frac{1}{4}\sum_{b\in\Lambda_{\mr{B}}}\left(\ket*{+,0}+\ket*{0,-}\right)_{b,b+1}\bigotimes_{b'\in\Lambda_{\mr{B}}\setminus\{b,b+1\}}\ket*{\what{+}}_{b'}=-N\frac{\sqrt{2}}{8}\ket*{S_N}+P_{\mr{Ryd}}\ket*{\delta\wtil{S}_N},
\end{equation}
where $\innerproduct*{\wtil{S}_N}{\delta\wtil{S}_N}=0$. Therefore, one can estimate $E_N\cong7\sqrt{2}N/8$. Indeed, for $N=10$ our estimation yields $E_N\cong70\sqrt{2}/8\cong12.37$, which is close to numerical value $E_N\cong12.07$.

For an estimation of $E_{N-1}$, we express $\ket*{S_{N-1}}$ as
\begin{equation}
    \ket*{S_{N-1}}=P_{\mr{Ryd}}\left(\ket*{\what{T}_{2,1}}_{b,b+1}\bigotimes_{b'\in\Lambda_{\mr{B}}\setminus\{b,b+1\}}\ket*{\what{+}}_{b'}+\sum_{b'\in\Lambda_{\mr{B}}\setminus\{b,b+1\}}\ket*{\what{T}_{2,2}}_{b,b+1}\otimes\ket*{\what{0}}_{b'}\bigotimes_{b''\in\Lambda_{\mr{B}}\setminus\{b,b+1,b'\}}\ket*{\what{+}}_{b''}\right).
\end{equation}
This relation holds for any $b\in\Lambda_{\mr{B}}$. Since $\innerproduct*{+,-}{\what{T}_{2,1}}=0$, we find
\begin{equation}\begin{split}
    H_1\ket*{\wtil{S}_{N-1}}&=-\frac{1}{4}\sum_{b\in\Lambda_{\mr{B}}}\sum_{b'\in\Lambda_{\mr{B}}\setminus\{b,b+1\}}\left(\ket*{+,0}+\ket*{0,-}\right)_{b,b+1}\otimes\ket*{\what{0}}_{b'}\bigotimes_{b''\in\Lambda_{\mr{B}}\setminus\{b,b+1,b'\}}\ket*{\what{+}}_{b''}\\
    &=-\frac{\sqrt{2}}{8}\sum_{b\in\Lambda_{\mr{B}}}\ket*{\what{T}_{2,2}}_{b,b+1}\otimes\ket*{\what{0}}_{b'}\bigotimes_{b''\in\Lambda_{\mr{B}}\setminus\{b,b+1,b'\}}\ket*{\what{+}}_{b''}+\ket*{\delta\wtil{S}_{N-1}}\\
    &=-(N-2)\frac{\sqrt{2}}{8}\ket*{\wtil{S}_{N-1}}+\ket*{\delta\wtil{S}_{N-1}},
    \end{split}
\end{equation}
where $\innerproduct*{\wtil{S}_{N-1}}{\delta\wtil{S}_{N-1}}=0$. Thus, one can estimate $E_{N-1}\cong(7N-6)\sqrt{2}/8$. For $N=10$, it is $11.37$, which is close the numerical value $E_{N-1}\cong11.10$. 
\section{Another set of trial wave functions}
In the main text, we consider the trial wave function $\ket*{S_n}$ that is viewed as the eigenstates of $H_{\mr{Z}}$ with the maximal spin number projected onto the constraint subspace. However, one can also construct another set of trial wave functions based on $\ket*{\Gamma}$. We consider
\begin{equation}\label{eq:another Sn}
    \ket*{S'_n}\coloneqq P_{\mr{Ryd}}\left(J^+\right)^n\ket*{\Gamma},
\end{equation}
where $J^\pm$ is defined in the main text. In fractional spin-$1/2$ representation, $\ket*{S'_n}$ is expressed as 
\begin{equation}
    \begin{split}
        \ket*{S'_n}&=\sum_{\{b_k\}_{k=1}^n\subset\Lambda_{\mr{B}}}P_{\mr{Ryd}}\msf{A}\bigotimes_{k=1}^n\ket*{\rightarrow\rightarrow}_{(b_k,\mr{R}),(b_k+1,\mr{L})}\bigotimes_{b'\in\Lambda_{\mr{B}}\setminus\{b_k\}_{k=1}^n}\frac{1}{\sqrt{2}}\left(\ket*{\uparrow\uparrow}-\ket*{\downarrow\downarrow}\right)_{(b',\mr{R}),(b'+1,\mr{L})}
    \end{split}
\end{equation}

We numerically observe that squared overlap $|\innerproduct*{S'_n}{\mc{S}^{\mr{PXP}}_n}|^2$ is roughly as large as $|\innerproduct*{S_n}{\mc{S}^{\mr{PXP}}_n}|^2$ as shown in Fig.~\ref{fig:overlap_MPs}. 
\begin{figure}
    \centering
    \includegraphics[width=.5\textwidth]{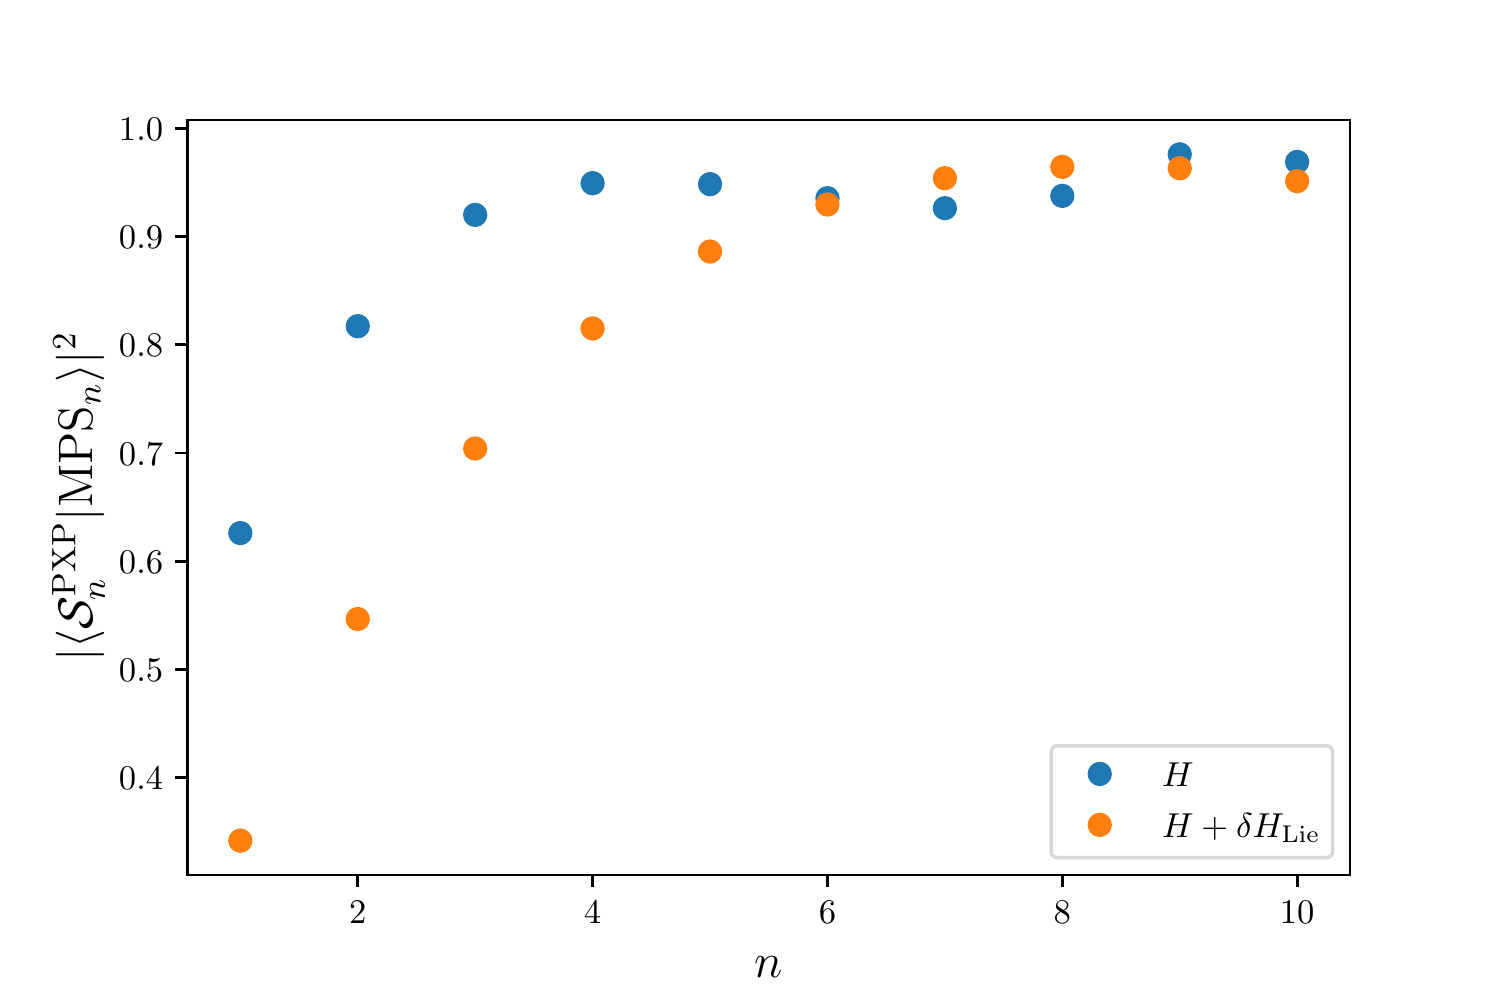}
    \caption{Squared overlap between the exact scar states $\ket*{\mc{S}_n^{\mr{PXP}}}$ and our trial wave functions $\ket*{S'_n}$, i.e., $|\innerproduct*{\mc{S}_n^{\mr{PXP}}}{S'_n}|^2$.}
    \label{fig:overlap_MPs}
\end{figure}

We use this ansatz to estimate the energy of $\ket*{\mc{S}_1}$. Using MPS representation, $\ket*{S'_1}$ is written as
\begin{equation}
    \ket*{S'_1}=\sum_{b\in\Lambda_{\mr{B}}}\sum_{\{\sigma_i\}_{i=1}^N\in\{\pm,0\}^{\otimes N}}P_{\mr{Ryd}}\left(\msf{v}_\rightarrow^{\sigma_b}\right)^{\mr{T}}\msf{A}^{\sigma_{[b+1]}}\cdots\msf{A}^{\sigma_{[b+N-2]}}\msf{w}_\rightarrow^{\sigma_{[b+N-1]}}\ket*{\sigma_1\cdots\sigma_N},
\end{equation}
where $[b]$ satisfies $b\equiv[b] (\mr{mod} N)$ and $1\leq [b]<N$. We also define $\ket*{\wtil{S}'_1}$ and $\ket*{M^{\rightarrow\rightarrow}_{b,b+1}}$ as
\begin{equation}\begin{split}
    \ket*{\wtil{S}'_1}&\coloneqq\sum_{b\in\Lambda_{\mr{B}}}\sum_{\{\sigma_i\}_{i=1}^N\in\{\pm,0\}^{\otimes N}}\left(\msf{v}_\rightarrow^{\sigma_b}\right)^{\mr{T}}\msf{A}^{\sigma_{[b+1]}}\cdots\msf{A}^{\sigma_{[b+N-2]}}\msf{w}_\rightarrow^{\sigma_{[b+N-1]}}\ket*{\sigma_1\cdots\sigma_N}\\
    \ket*{M^{\rightarrow\rightarrow}_{b,b+1}}&\coloneqq\sum_{\{\sigma_i\}_{i=1}^N\in\{\pm,0\}^{\otimes N}}\left(\msf{v}_\rightarrow^{\sigma_b}\right)^{\mr{T}}\msf{A}^{\sigma_{[b+1]}}\cdots\msf{A}^{\sigma_{[b+N-2]}}\msf{w}_\rightarrow^{\sigma_{[b+N-1]}}\ket*{\sigma_1\cdots\sigma_N}\\
    &=\msf{A}\ket*{\rightarrow\rightarrow}_{(b,\mr{R}),(b+1,\mr{L})}\bigotimes_{b'\in\Lambda_{\mr{B}}\setminus\{b\}}\frac{1}{\sqrt{2}}\left(\ket*{\uparrow\uparrow}-\ket*{\downarrow\downarrow}\right)_{(b',\mr{R}),(b'+1,\mr{L})},
    \end{split}
\end{equation}
so that $P_{\mr{Ryd}}\ket*{\wtil{S}'_1}=\ket*{S'_1}$ and $\ket*{\wtil{S}'_1}=\sum_{b\in\Lambda_{\mr{B}}}\ket*{M^{\rightarrow\rightarrow}_{b,b+1}}$.
We find
\begin{equation}\label{eq:H|S'1>}\begin{split}
    H\ket*{S'_1}&=\sqrt{2}\ket*{S'_1}-\sum_{b\in\Lambda_{\mr{B}}}P_{\mr{Ryd}}\left(\ket*{+,0}+\ket*{0,-}\right)\bra*{+,-}_{b,b+1}\ket*{M^{\rightarrow\rightarrow}_{b,b+1}}\\
    &=\sqrt{2}\ket*{S'_1}+\frac{1}{4}\sum_{b\in\Lambda_{\mr{B}}}\left(\ket*{+,0}+\ket*{0,-}\right)_{b,b+1}\otimes\ket*{M^{\uparrow\downarrow}_{b-1,b+2}},
    \end{split}
\end{equation}
where
\begin{equation}
    \begin{split}
        \ket*{M_{b-1,b+2}^{\uparrow\downarrow}}\coloneqq\left(\bigotimes_{b'\in\Lambda_{\mr{B}}\setminus\{b,b+1\}}A_{b'}\right)\ket*{\uparrow\downarrow}_{(b-1,\mr{R}),(b+2,\mr{L})}\bigotimes_{b''\in\Lambda_{\mr{B}}\setminus\{b-1,b,b+1\}}\frac{1}{\sqrt{2}}\left(\ket*{\uparrow\uparrow}-\ket*{\downarrow\downarrow}\right)_{(b'',\mr{R}),(b''+1,\mr{L})}.
    \end{split}
\end{equation}
MPS representation of $\ket*{M^{\uparrow\downarrow}_{b-1,b+2}}$ is as follows:
\begin{equation}
    \ket*{M_{b-1,b+2}^{\uparrow\downarrow}}=\sum_{\{\sigma_i\}_{i\in\Lambda_{B}\setminus\{b,b+1\}}\in\{\pm,0\}^{\otimes N-2}}\left(\msf{v}^{\sigma_{[b+2]}}_\downarrow\right)^{\mr{T}}\msf{A}^{\sigma_{[b+3]}}\cdots\msf{A}^{\sigma_{[b-2]}}\msf{w}_\uparrow^{\sigma_{[b-1]}}\ket*{\sigma_1\cdots\sigma_{N}},
\end{equation}
where we do not include $\sigma_b$ and $\sigma_{b+1}$ in the summation. Here, we define the boundary vectors as $\msf{v}_\downarrow^\sigma\coloneqq(\msf{v}^\sigma_\rightarrow-\msf{v}^\sigma_\leftarrow)/\sqrt{2}$ and $\msf{w}^\sigma_\uparrow\coloneqq(\msf{w}^\sigma_\rightarrow+\msf{w}^\sigma_\leftarrow)/\sqrt{2}$. We also define the second term of the second line in Eq.~\eqref{eq:H|S'1>} as $\ket*{\delta S'_1}$, i.e., $H\ket*{S'_1}=\sqrt{2}\ket*{S'_1}+\frac{1}{4}\ket*{\delta S'_1}$. Thus, the energy of $\ket*{S'_1}$ is evaluated as 
\begin{equation}\label{eq:renormalized H|S'1>}
    H\ket*{S'_1}=\left(\sqrt{2}+\frac{1}{4}\frac{\innerproduct*{S'_1}{\delta S'_1}}{\innerproduct*{S'_1}{S'_1}}\right)\ket*{S'_1}+\ket*{S'_\perp},
\end{equation}
where $\ket*{S'_\perp}$ satisfies $\innerproduct*{S'_1}{S'_\perp}=0$. As both $\ket*{S'_1}$ and $\ket*{\delta S'_1}$ can be expressed as MPS, one can calculate their norm and inner product, though complicated computations are necessary. We omit a detailed derivation, but one finds at large $N$,
\begin{equation}
    \innerproduct*{S'_1}\cong\frac{14N}{9}\left(\frac{3}{4}\right)^N,\,\,\innerproduct*{S'_1}{\delta S'_1}\cong-\frac{4\sqrt{2}N}{9}\left(\frac{3}{4}\right)^N.
\end{equation}
Thus, for large $N$, we obtain $\sqrt{2}+\frac{1}{4}\frac{\innerproduct*{S'_1}{\delta S'_1}}{\innerproduct*{S'_1}}\cong\frac{13}{14}\sqrt{2}\cong1.3132$, which is close to the empirical value ($\cong1.33$).

Moreover, one can estimate $\norm*{\ket*{S'_\perp}}$ and obtain $\norm*{\ket*{S'_\perp}}/\norm*{\ket*{S'_1}}=\sqrt{151/(3\cdot14^3)}\cong0.1354$ in the thermodynamic limit.  

We note that this ansatz is not a good approximation once the perturbations are added (Fig.~\ref{fig:overlap_MPs}).
\section{Estimate of the optimal coefficient of the perturbation}
We have obtained the optimal coefficient of the perturbation $\delta H(\lambda)$ in the main text. Here we derive it in a detail. Our idea is to minimize $\sum_n\norm*{(H_1+\delta H(\lambda))\ket*{\wtil{S}_n}}^2$ with respect to $\lambda$, instead of $\sum_n\norm*{P_{\mr{Ryd}}(H_1+\delta H(\lambda))\ket*{S_n}}^2$, assuming that they are not so different. 
\subsection{The scar states}
Our trial wave function $\ket{S_n}$ for the scar states is given as follows,
\begin{equation}\begin{split}
    \ket{S_n}&=P_{\mr{Ryd}}\ket*{\wtil{S}_n}=P_{\mr{Ryd}}\left(J^-\right)^{N-n}\bigotimes_{b\in\Lambda_{\mr{B}}}\ket*{\what{+}}_b
    \\
    J^\pm&=\sqrt{2}\sum_{b\in\Lambda_{\mr{B}}}\left(\dyad*{\what{\pm}}{\what{0}}+\dyad*{\what{0}}{\what{\mp}}\right)_b.
    \end{split}
\end{equation}
We split the collective spin-raising (lowering) operator as
\begin{equation}\begin{split}
    J^\pm&=J_{b,b+1}^\pm+J_{\Lambda_{\mr{B}}\setminus\{b,b+1\}}^\pm\\
    J_{b,b+1}^\pm&\coloneqq\sqrt{2}\left(\dyad*{\what{\pm}}{\what{0}}+\dyad*{\what{0}}{\what{\mp}}\right)_b+\sqrt{2}\left(\dyad*{\what{\mp}}{\what{0}}+\dyad*{\what{0}}{\what{\mp}}\right)_{b+1}\\
    J^\pm_{\Lambda_{\mr{B}}\setminus\{b,b+1\}}&\coloneqq\sqrt{2}\sum_{b'\in\Lambda_{\mr{B}}\setminus\{b,b+1\}}\left(\dyad*{\what{\pm}}{\what{0}}+\dyad*{\what{0}}{\what{\mp}}\right)_{b'}.
    \end{split}
\end{equation}
Using these operators, we can write $\ket*{\wtil{S}_{N-n}}$ with $n\geq3$ as
\begin{equation}\begin{split}
    \ket*{\wtil{S}_{N-n}}&=\sum_{k=0}^4\binom{n}{k}\left(J^-_{b,b+1}\right)^k\ket*{\what{T}_{2,2}}_{b,b+1}\otimes\left(J^-_{\Lambda_{\mr{B}}\setminus\{b,b+1\}}\right)^{n-k}\ket*{\what{T}_{N-2,N-2}}_{\Lambda_{\mr{B}}\setminus\{b,b+1\}}\\
    &=c\ket*{\what{T}_{2,2}}_{b,b+1}\otimes\ket*{\what{T}_{N-2,N-n-2}}_{\Lambda_{\mr{B}}\setminus\{b,b+1\}}+2c\sqrt{\frac{n}{-n+2N-3}}\ket*{\what{T}_{2,1}}_{b,b+1}\otimes\ket*{\what{T}_{N-2,N-n-1}}_{\Lambda_{\mr{B}}\setminus\{b,b+1\}}\\
    &+c\sqrt{\frac{3n!(-n+2N-4)!}{2(n-2)!(-n+2N-2)!}}\ket*{\what{T}_{2,0}}_{b,b+1}\otimes\ket*{\what{T}_{N-2,N-n}}_{\Lambda_{\mr{B}}\setminus\{b,b+1\}}\\
    &+c\sqrt{\frac{n!(-n+2N-4)!}{6(n-3)!(-n+2N-1)!}}\ket*{\what{T}_{2,-1}}_{b,b+1}\otimes\ket*{\what{T}_{N-2,N-n+1}}_{\Lambda_{\mr{B}}\setminus\{b,b+1\}}\\
    &+c\sqrt{\frac{n!(-n+2N-4)!}{(n-4)!(-n+2N)!}}\ket*{\what{T}_{2,-2}}_{b,b+1}\otimes\ket*{\what{T}_{N-2,N-n+2}}_{\Lambda_{\mr{B}}\setminus\{b,b+1\}},
    \end{split}
\end{equation}
where $c\coloneqq\prod_{M=N-n-1}^{N-2}\sqrt{(N-2)(N-1)-M(M-1)}$. Here, $\ket*{\what{T}_{S,M}}$ is a composite state with total spin $S$ and $S^x=M$. When $N$ is sufficiently large, one can approximate $\ket*{\wtil{S}_n}$ as
\begin{equation}\label{eq:|Sn> approximate}
    \begin{split}
        \frac{1}{c}\ket*{\wtil{S}_{N-n}}&\cong \ket*{\what{T}_{2,2}}_{b,b+1}\otimes\ket*{\what{T}_{N-2,N-n-2}}_{\Lambda_{\mr{B}}\setminus\{b,b+1\}}+2\sqrt{\frac{s}{2-s}}\ket*{\what{T}_{2,1}}_{b,b+1}\otimes\ket*{\what{T}_{N-2,N-n-1}}_{\Lambda_{\mr{B}}\setminus\{b,b+1\}}\\
        &+\sqrt{\frac{3}{2}}\frac{s}{2-s}\ket*{\what{T}_{2,0}}_{b,b+1}\otimes\ket*{\what{T}_{N-2,N-n}}_{\Lambda_{\mr{B}}\setminus\{b,b+1\}}+\sqrt{\frac{s^3}{6(2-s)^3}}\ket*{\what{T}_{2,-1}}_{b,b+1}\otimes\ket*{\what{T}_{N-2,N-n+1}}_{\Lambda_{\mr{B}}\setminus\{b,b+1\}}\\
        &+\frac{1}{12}\frac{s^2}{(2-s)^2}\ket*{\what{T}_{2,-2}}_{b,b+1}\otimes\ket*{\what{T}_{N-2,N-n+2}}_{\Lambda_{\mr{B}}\setminus\{b,b+1\}},
    \end{split}
\end{equation}
where $s\coloneqq n/N$. Each coefficient is plotted in Fig.~[FIG]. When $n$ is small, the dominant contribution in $\ket*{\wtil{S}_{N-n}}$ is $\ket*{\what{T}_{2,2}}_{b,b+1}$, but as $n$ increases $\ket*{\what{T}_{2,1}}_{b,b+1}$ and $\ket*{\what{T}_{2,0}}_{b,b+1}$ become dominant. For later argument, we define the reduced density matrix $\rho_S$ for the states $\ket*{\wtil{S}_n}$ as 
\begin{equation}
    \rho_S\coloneqq\frac{1}{N}\sum_{n=1}^N\mr{Tr}_{\Lambda_{\mr{B}}\setminus\{b,b+1\}}\frac{1}{\norm*{\ket*{\wtil{S}_n}}^2}\dyad*{\wtil{S}_n},
\end{equation}
where $\mr{Tr}_{\Lambda_{\mr{B}}\setminus\{b,b+1\}}$ is partial trace on $\Lambda_{\mr{B}}\setminus\{b,b+1\}$. We can approximately obtain $\rho_S$ using Eq.~\eqref{eq:|Sn> approximate} as
\begin{equation}
    \begin{split}
        \rho_S&\cong\frac{1}{N}\sum_{s=1/N}^{1}\frac{1}{Z(s)}\left(P^{(2,2)}_{b,b+1}+\frac{4s}{2-s}P^{(2,1)}_{b,b+1}+\frac{3s^2}{2(2-s)^2}P^{(2,0)}_{b,b+1}+\frac{s^3}{6(2-s)^3}P^{(2,-1)}_{b,b+1}+\frac{s^4}{144(2-s)^4}P^{(2,-2)}_{b,b+1}\right)\\
        Z(s)&\coloneqq1+\frac{4s}{2-s}+\frac{3s^2}{2(2-s)^2}+\frac{s^3}{6(2-s)^3}+\frac{s^4}{144(2-s)^4},
    \end{split}
\end{equation}
where $P_{b,b+1}^{(S,M)}\coloneqq\dyad*{\what{T}_{S,M}}_{b,b+1}$. Note that we can approximate $\rho_S$ further by replacing $N^{-1}\sum_{s=1/N}^1\rightarrow\int_0^1ds$.
\begin{figure}
    \centering
    \includegraphics[width=.5\textwidth]{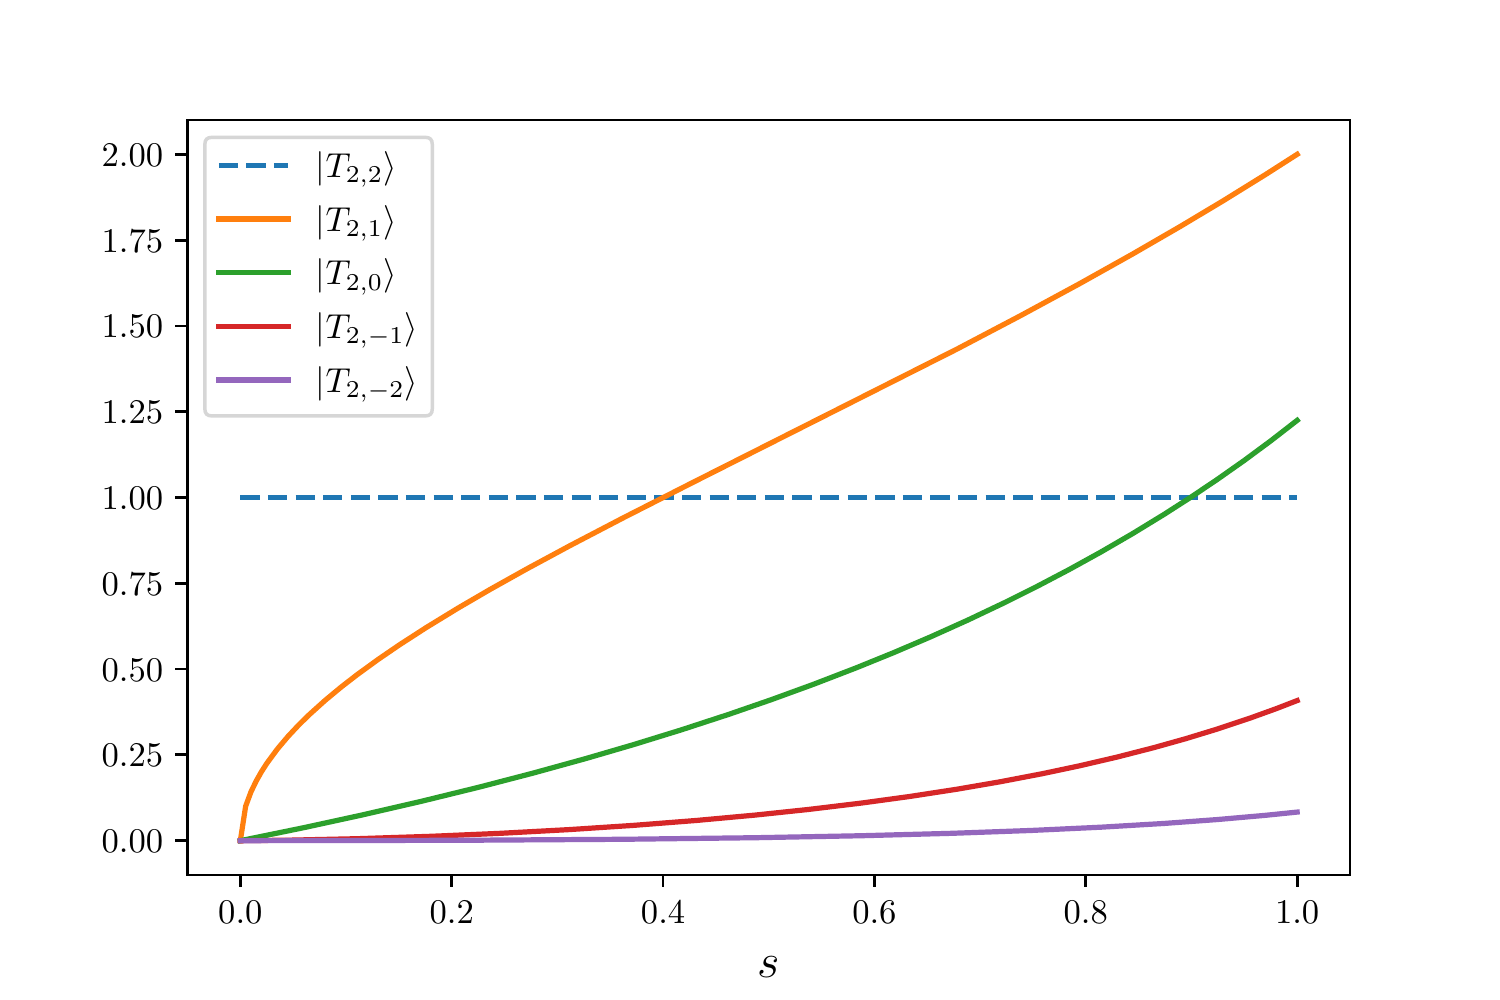}
    \caption{Coefficients of $\ket*{\what{T}_{2,M}} (-2\leq M\leq 2)$ in Eq.~\eqref{eq:|Sn> approximate} as functions of $s$.}
    \label{fig:coeffs}
\end{figure}
%\subsection{Another trial wave functions}
\subsection{The estimate of the optimal coefficient}
As shown in the main text, we have found 
\begin{equation}
    \begin{split}
        (H+\delta H(\lambda))\ket*{S_n}&=P_{\mr{Ryd}}\left(H_{\mr{Z}}+H_{\mr{rem}}(\lambda)\right)\ket*{\wtil{S}_n}\\
        H_{\mr{rem}}(\lambda)&=\sum_{b\in\Lambda_{\mr{B}}}h_{b,b+1}(\lambda)\\
        h_{b,b+1}(\lambda)&=\frac{-1+2\lambda}{\sqrt{6}}\left(\ket*{+,0}+\ket*{0,-}\right)\bra*{T_{2,0}}_{b,b+1}+\frac{\lambda}{\sqrt{2}}\ket*{0,0}\left(\bra*{T_{2,1}}+\bra*{T_{2,-1}}\right)_{b,b+1}.
    \end{split}
\end{equation}
We find
\begin{equation}
    h_{b,b+1}^\dag(\lambda)h_{b,b+1}(\lambda)=\frac{(-1+2\lambda)^2}{3}\dyad*{T_{2,0}}_{b,b+1}+\frac{\lambda^2}{2}\left(\ket*{T_{2,1}}+\ket*{T_{2,-1}}\right)\left(\bra*{T_{2,1}}+\bra*{T_{2,-1}}\right)_{b,b+1}.
\end{equation}
As $\ket*{T_{2,0}}=\sqrt{3/8}\ket*{\what{T}_{2,2}}-1/2\ket*{\what{T}_{2,0}}+\sqrt{3/8}\ket*{\what{T}_{2,-2}}$ and $\ket*{T_{2,1}}+\ket*{T_{2,-1}}=\ket*{\what{T}_{2,2}}-\ket*{\what{T}_{2,-2}}$, we find
\begin{equation}
    \begin{split}
        \mr{Tr}_{\{b,b+1\}}\rho_Sh^\dag_{b,b+1}(\lambda)h_{b,b+1}(\lambda)&=\frac{(-1+2\lambda)^2}{3}\left(\frac{3}{8}\expval*{\rho_S}{\what{T}_{2,2}}+\frac{1}{4}\expval*{\rho_S}{\what{T}_{2,0}}+\frac{3}{8}\expval*{\rho_S}{\what{T}_{2,-2}}\right)\\
        &+\frac{\lambda^2}{2}\left(\expval*{\rho_S}{\what{T}_{2,2}}+\expval*{\rho_S}{\what{T}_{2,-2}}\right)\\
        &\cong\frac{1}{N}\sum_{s=1/N}^1\left[\frac{(-1+2\lambda)^2}{8Z(s)}\left(1+\frac{s^2}{(2-s)^2}+\frac{s^4}{144(2-s)^4}\right)+\frac{\lambda^2}{2Z(s)}\left(1+\frac{s^4}{144(2-s)^4}\right)\right]\\
        &\cong\int_0^1ds\left[\frac{(-1+2\lambda)^2}{8Z(s)}\left(1+\frac{s^2}{(2-s)^2}+\frac{s^4}{144(2-s)^4}\right)+\frac{\lambda^2}{2Z(s)}\left(1+\frac{s^4}{144(2-s)^4}\right)\right],
    \end{split}
\end{equation}
where $\mr{Tr}_{\{b,b+1\}}$ is partial trace on $\{b,b+1\}$. This function becomes smallest at $\lambda=\alpha/(2(\alpha+\beta))$, where
\begin{equation}\label{eq:alpha, beta}
    \begin{split}
        \alpha&\coloneqq\int_0^1ds\frac{1}{Z(s)}\left(1+\frac{s^2}{(2-s)^2}+\frac{s^4}{144(2-s)^4}\right)\cong0.5350\\
        \beta&\coloneqq\int_0^1ds\frac{1}{Z(s)}\left(1+\frac{s^4}{144(2-s)^4}\right)\cong0.4739.
    \end{split}
\end{equation}
Thus, we numerically find the optimal coefficient $\lambda\cong0.2651$. We define integrands in Eq.~\eqref{eq:alpha, beta} as $\alpha(s)$ and $\beta(s)$, i.e., $\alpha=\int_0^1ds\alpha(s), \beta=\int_0^1ds\beta(s)$ and plot them in Fig.~\ref{fig:integrand}.
\begin{figure}
    \centering
    \includegraphics[width=.5\textwidth]{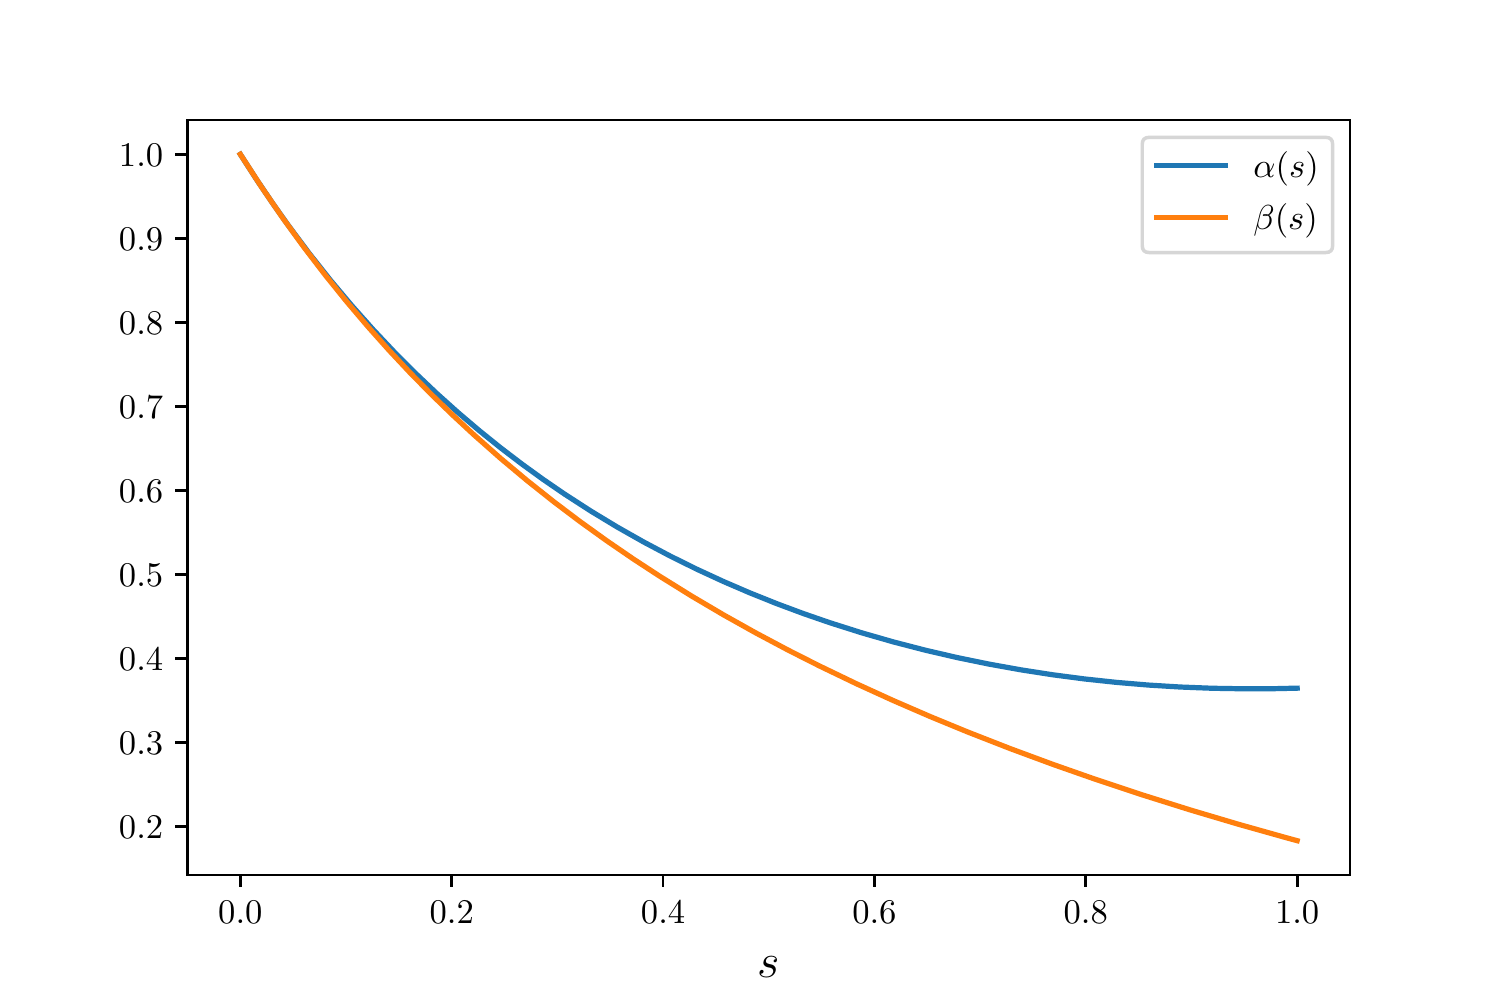}
    \caption{Integrands in Eq.~\eqref{eq:alpha, beta} $\alpha(s)$ and $\beta(s)$ as functions of $s$.}
    \label{fig:integrand}
\end{figure}
\section{A possible way to generate a sequence of Hermitian perturbations}
In the main text, we discussed the non-Hermitian perturbation which makes our trial states $\ket*{S_n}$ exact, and the Hermitian perturbation which makes $\ket*{S_n}$ close to an exact eigenstate. However, in the literature, the recipes to generate perturbations allow infinitely many terms with vanishing coefficients for long-range ones. Here we show a possible way to generate a sequence of Hermitian perturbations. We will show neither that this sequence converges in some operator norm sense, nor that any numerical result which could support the convergence.

Our idea is simple: given that we obtain a proper non-Hermitian perturbation $H_{\mr{NH}}$, in order to have a Hermitian operator, one has to add its Hermitian conjugate, i.e., $H_{\mr{NH}}+H_{\mr{NH}}^\dag$. However, this operator does not completely cancel $H_1$. Namely, we could have non-vanishing vectors $P_{\mr{Ryd}}(H_1+H_{\mr{NH}}+H_{\mr{NH}}^\dag)\ket*{\wtil{S}_n}=P_{\mr{Ryd}}H_{\mr{NH}}^\dag\ket*{\wtil{S}_n}\not=0$ for some $n$. Therefore, we should repeat the same procedure by replacing $H_1$ with $H_{\mr{NH}}^\dag$, which leads to another non-Hermitian operator $H'_{\mr{NH}}$ such that $P_{\mr{Ryd}}\left(H_{\mr{NH}}^\dag+H'_{\mr{NH}}\right)\ket*{\wtil{S}_n}=0$. From this non-Hermitian operator $H'_{\mr{NH}}$, we construct a Hermitian operator $H'_{\mr{NH}}+H'^\dag_{\mr{NH}}$. We essentially repeat this procedure. Therefore, we might obtain infinitely many terms, but with vanishing coefficients.
\subsection{The first step}
From the argument in the main text, any operator of a form
\begin{equation}
    H'_{\mr{NH}}=\sum_{b\in\Lambda}\left(\ket*{+,0}+\ket*{0,-}\right)\bra{\chi}_{b,b+1},
\end{equation}
where
\begin{equation}
    \ket*{\chi}=\frac{1}{\sqrt{6}}\ket*{T_{2,0}}+\sum_{S<2}\sum_{M=-S}^Sc_{S,M}\ket*{T_{S,M}},
\end{equation}
annihilate $H_1$, i.e., $P_{\mr{Ryd}}\left(H_1+H'_{\mr{NH}}\right)\ket*{\wtil{S}_n}=0$ as long as $H'_{\mr{NH}}$ commutes with $P_{\mr{Ryd}}$. We now relax this condition: instead of requiring that $H'_{\mr{NH}}$ should commute with $P_{\mr{Ryd}}=\prod_{b\in\Lambda_{\mr{B}}}(1-\dyad*{+,-})_{b,b+1}$, we require that $H'_{\mr{NH}}$ should commute with $(1-\dyad*{+,-})_{b,b+1}$. This condition allows us to make more options for $\ket*{\chi}$. Indeed, the following parametrized state $\ket*{\chi(a)}$ satisfies this condition,
\begin{equation}
    \ket*{\chi(a)}=\frac{1-a}{2}\ket*{0,0}+a\ket*{-,+},
\end{equation}
where $a$ is a parameter. This state has the smallest norm when $a=1/5$. Thus, we obtain 
\begin{equation}
    H'_{\mr{NH}}=\frac{2}{5}\sum_{b\in\Lambda_{\mr{B}}}\left(\ket*{+,0}+\ket*{0,-}\right)\bra*{0,0}_{b,b+1}+\frac{1}{5}\sum_{b\in\Lambda_{\mr{B}}}\left(\right)\bra*{-,+}_{b,b+1}.
\end{equation}
Note that the second term does not commute with $P_{\mr{Ryd}}$. However, we can make $H'_{\mr{NH}}$ commute with $P_{\mr{Ryd}}$ by adding suitable projection operators such that the second term becomes
\begin{equation}
    \frac{1}{5}\sum_{b\in\Lambda_{\mr{B}}}\left(1-\dyad*{+}\right)_{b-1}\left(\ket*{+,0}+\ket*{0,-}\right)\bra*{-,+}_{b,b+1}\left(1-\dyad*{-}\right)_{b+2}.
\end{equation}
Here, we add the suitable projection operators $(1-\dyad*{+})_{b-1}$ and $(1-\dyad*{-})_{b+2}$ onto the constrained subspace. Thus our non-Hemritian perturbation is
\begin{equation}
    \delta_1H_{\mr{NH}}=\frac{2}{5}\sum_{b\in\Lambda_{\mr{B}}}\left(\ket*{+,0}+\ket*{0,-}\right)\bra*{0,0}_{b,b+1}+\frac{1}{5}\sum_{b\in\Lambda_{\mr{B}}}\left(1-\dyad*{+}\right)_{b-1}\left(\ket*{+,0}+\ket*{0,-}\right)\bra*{-,+}_{b,b+1}\left(1-\dyad*{-}\right)_{b+2}.
\end{equation}
Note that $\delta_1H_{\mr{NH}}$ does not cancel $H_1$ completely. Instead we have
\begin{equation}
    \begin{split}
        &P_{\mr{Ryd}}\left(H_1+\delta_1H_{\mr{NH}}\right)\ket*{\wtil{S}_n}=P_{\mr{Ryd}}H'_{\mr{rem};1}\ket*{\wtil{S}_n}\\
        &H'_{\mr{rem};1}=-\frac{1}{5}\sum_{b\in\Lambda_{\mr{B}}}\left(\ket*{+,+,0}+\ket*{+,0,-}\right)\bra*{+,-,+}_{b,b+1,b+2}-\frac{1}{5}\sum_{b\in\Lambda_{\mr{B}}}\left(\ket*{+,0,-}+\ket*{0,-,-}\right)\bra*{-,+,-}_{b,b+1,b+2}\\
        &+\frac{1}{5}\sum_{b\in\Lambda_{\mr{B}}}\left(\ket*{+,+,0,-}+\ket*{+,0,-,-}\right)\bra*{+,-,+,-}_{b,b+1,b+2,b+3}.
    \end{split}
\end{equation}
Our ``first-order" perturbation is $\delta_1H\coloneqq\delta_1H_{\mr{NH}}+\delta_1H_{\mr{NH}}^\dag$. Thus, we obtain $P_{\mr{Ryd}}\left(H_1+\delta_1H\right)\ket*{\wtil{S}_n}=P_{\mr{Ryd}}\left(\delta H_{\mr{NH}}^\dag+H'_{\mr{rem};1}\right)\ket*{\wtil{S}_n}$ and define $H_{\mr{rem};1}\coloneqq H_{\mr{NH}}^\dag+H'_{\mr{rem};1}$.
\subsection{The second step}
We repeat the same procedure by regarding $H_{\mr{rem};1}$ as $H_1$, i.e., we try to find a non-Hermitian operator $\delta_2H_{\mr{NH}}$ such that $P_{\mr{Ryd}}\left(H_{\mr{rem};1}+\delta_2H_{\mr{NH}}\right)\ket*{\wtil{S}_n}=0$. Since it is lengthy but not instructive to consider all the terms in $H_{\mr{rem};1}$, we focus only on the operator 
\begin{equation}\label{eq:part}
    A\coloneqq\frac{2}{5}\sum_{b\in\Lambda_{\mr{B}}}\ket*{0,0}\left(\bra*{+,0}+\bra*{0,-}\right)_{b,b+1},
\end{equation}
which is included in $\delta_1H_{\mr{NH}}^\dag$. More precisely, we try to find an operator $A'_{\mr{NH}}$ satisfying $P_{\mr{Ryd}}(A+A'_{\mr{NH}})\ket*{\wtil{S}_n}=0$ and make $A'_{\mr{NH}}$ commute with $P_{\mr{Ryd}}$. It is easy to find
\begin{equation}
    \ket*{+,0}+\ket*{0,-}=\frac{1}{\sqrt{2}}\ket*{T_{2,1}}+\frac{1}{\sqrt{2}}\ket*{T_{2,-1}}+\frac{1}{\sqrt{2}}\ket*{T_{1,1}}+\frac{1}{\sqrt{2}}\ket*{T_{1,-1}}.
\end{equation}
As $\dyad*{0,0}{T_{1,\pm1}}$ annihilates $\ket*{\wtil{S}_n}$, we should consider the following operator: 
\begin{equation}\label{eq:counter term}
    A'_{\mr{NH}}=-\frac{2}{5\sqrt{2}}\sum_{b\in\Lambda_{\mr{B}}}\ket*{0,0}\left(\bra*{T_{2,1}}+\bra*{T_{2,-1}}\right)_{b,b+1}=-\frac{1}{5}\sum_{b\in\Lambda_{\mr{B}}}\ket*{0,0}\left(\bra*{+,0}+\bra*{0,+}+\bra*{0,-}+\bra*{-,0}\right)_{b,b+1}.
\end{equation}
This operator obviously satisfies $P_{\mr{Ryd}}(A+A'_{\mr{NH}})\ket*{\wtil{S}_n}=0$, although $A'_{\mr{NH}}$ does not commute with $P_{\mr{Ryd}}$.
We again add suitable projection operators so that Eq.~\eqref{eq:counter term} becomes
\begin{equation}
    A_{\mr{NH}}=-\frac{1}{5}\sum_{b\in\Lambda_{\mr{B}}}\ket*{0,0}\left(\bra*{+,0}\bra*{0,-}\right)_{b,b+1}-\frac{1}{5}\sum_{b\in\Lambda_{\mr{B}}}\dyad*{0,0}{0,+}_{b,b+1}\left(1-\dyad*{-}\right)_{b+2}-\frac{1}{5}\sum_{b\in\Lambda_{\mr{B}}}\left(1-\dyad*{+}\right)_b\dyad*{0,0}{-,0}_{b+1,b+2}.
\end{equation}
\subsection{A general step}
We generalize the steps above. Let us assume that we have $k$-(Hermitian) perturbations $\delta_1H,\cdots,\delta_kH$, and that we have $P_{\mr{Ryd}}\left(H_1+\sum_{i=1}^i\delta_kH\right)\ket*{\wtil{S}_n}=P_{\mr{Ryd}}H_{\mr{rem};k}\ket*{\wtil{S}_n}$. We assume that $H_{\mr{rem};k}$ is written as
\begin{equation}
    H_{\mr{rem};k}=\sum_{\mu=1}^{n_k}g_{k,\mu}\sum_{b\in\Lambda_{\mr{B}}}\dyad*{\varphi_{k,\mu}}{\pi_{k,\mu}}_{b,b+1,\cdots,b+i_{k,\mu}-1},
\end{equation}
where $\mu$ labels different terms and $g_{k,\mu}$ is a coefficient of a corresponding term. For simplicity, we also assume that $\ket*{\varphi_{k,\mu}}$ is a product state in the basis $\{\ket*{\pm},\ket*{0}\}^{\otimes i_{k,\mu}}$. $\ket*{\pi_{k,\mu}}$ does not have to be a product state. Instead, we choose $\ket*{\chi_{k,\mu}}$ such that the number of terms $n_k$ is minimized. 
We first express $\ket*{\chi_{k,\mu}}$ with respect to $\ket*{T_{S,M}}$,
\begin{equation}
    \ket*{\pi_{k,\mu}}_{1,\cdots,i_{k,\mu}-1}=\sum_S^{i_{k,\mu}}\sum_{M=-S}^Sc_{S,M}\ket*{T_{S,M}}_{1,\cdots,i_{k,\mu}-1},
\end{equation}
where $c_{S,M}$ is a coefficient. We try to find states $\ket*{\chi_{k,\mu}}$ such that
\begin{equation}\begin{split}
    &\ket*{\chi_{k,\mu}}_{1,\cdots,i_{k,\mu}-1}=\sum_{M=-i_{k,\mu}}^{i_{k,\mu}}c_{i_{k,\mu},M}\ket*{T_{i_{k,\mu},M}}_{1,\cdots,i_{k,\mu}-1}+\sum_{S\not=i_{k,\mu}}\sum_{M'=-S}^Sd_{S,M'}\ket*{T_{S,M'}}_{1,\cdots,i_{k,\mu}-1}\\
    &\prod_{l=1}^{i_{k,\mu}-1}\left(1-\dyad*{+,-}\right)_{l,l+1}\ket*{\chi_{k,\mu}}_{1,\cdots,i_{k,\mu}-1}=+\ket*{\chi_{k,\mu}}_{1,\cdots,i_{k,\mu}-1},
    \end{split}
\end{equation}
where $d_{S,M'}$ is another coefficient. Namely, we consider states with the same maximal total spin component. The second line is necessary to ensure that $\dyad*{\varphi_{k,\mu}}{\chi_{k,\mu}}$ commutes with $P_{\mr{Ryd}}$. 

If there are more than one choice for $\ket*{\chi_{k,\mu}}$ with $d_{S,M}<c_{S,M}$ for some $S,M$, then we choose $\ket*{\chi_{k,\mu}}$ with the smallest norm. Then, our non-Hermitian perturbation is 
\begin{equation}
    \delta_{k+1}H_{\mr{NH}}=-\sum_{\mu=1}^{n_k}g_{k,\mu}\sum_{b\in\Lambda_{\mr{B}}}\dyad*{\varphi_{k,\mu}}{\chi_{k,\mu}}_{b,b+1,\cdots,b+i_{k,\mu}-1},
\end{equation}
and our Hermitian perturbation becomes $\delta_{k+1}H=\delta_{k+1}H_{\mr{NH}}+\delta_{k+1}H_{\mr{NH}}^\dag$.

If there is no choice for $\ket*{\chi_{k,\mu}}$ except for $\ket*{\chi_{k,\mu}}=\ket*{\pi_{k,\mu}}$, we insert the identity $id=\dyad*{+}+\dyad*{0}+\dyad*{-}$ such that
\begin{equation}
    \dyad*{\varphi_{k,\mu}}{\pi_{k,\mu}}_{b,\cdots,b+i_{k,\mu}-1}=\dyad*{\varphi_{k,\mu}}{\pi_{k,\mu}}_{b,\cdots,b+i_{k,\mu}-1}\left(\dyad*{+}+\dyad*{0}+\dyad*{-}\right)_{b+i_{k,\mu}},
\end{equation}
and we do the same process for each operator, i.e., $\dyad*{\varphi_{k,\mu}}{\pi_{k,\mu}}_{b,\cdots,b+i_{k,\mu}-1}\dyad*{\alpha}_{b+i_{k,\mu}}$ for $\alpha=\pm,0$.

%\bibliography{reference_SM}
